# Supplementary material for: Interplay of chiral and helical states in a Quantum Spin Hall Insulator lateral junction
Source: arXiv:1702.08561 ancillary file (2017-12-13)
Supplement: Supplementary file 1 [file edge-states-interplay_SM.pdf]

# Supplemental Materials: Interplay of chiral and helical states in a Quantum Spin Hall Insulator lateral junction

M. R. Calvo,[1,2,3,4,*] F. de Juan,[5,†] R. Ilan,[6,5] E. J. Fox,[1,2] A. J. Bestwick,[1,2] M. Mühlbauer,[7] J. Wang,[1,2,8] C. Ames,[7] P. Leubner,[7] C. Brüne,[7] S. C. Zhang,[1,2] H. Buhmann,[7] L. W. Molenkamp,[7] and D. Goldhaber-Gordon[1,2,‡]

[1] *Department of Physics, Stanford University, Stanford, California 94305, USA*
[2] *Stanford Institute for Materials and Energy Sciences, SLAC National Accelerator Laboratory, Menlo Park, California 94025, USA*
[3] *CIC nanoGUNE, 20018 Donostia-San Sebastian, Spain*
[4] *Ikerbasque, Basque Foundation for Science, 48013 Bilbao, Spain*
[5] *Department of Physics, University of California, Berkeley, California 94720, USA*
[6] *Raymond and Beverly Sackler School of Physics and Astronomy, Tel Aviv University, Tel Aviv 69978, Israel*
[7] *Physikalisches Institut (EP3) and Röntgen Center for Complex Material Systems, Universität Würzburg, Am Hubland, 97074 Würzburg, Germany*
[8] *State Key Laboratory of Surface Physics and Department of Physics, Fudan University, Shanghai 200433, China*

(Dated: December 13, 2017)

## S1. Methods

The material layer structure is sketched in Fig. S1 (for material growth details see Ref. [S1]). An n++ doped GaAs substrate serves as a backgate electrode. The 4 $\mu$m relaxed CdTe buffer layer sets the lattice constant for the top layers. The strained HgTe quantum well thickness is $8.0 \pm 0.5$ nm extracted by x-ray reflectivity. This exceeds the critical thickness for strained HgTe (estimated to be 6.7 nm following a similar approach to Ref. [S2]), so we expect an inverted band structure and QSH edge states. We fabricate 10 $\mu$m wide Hall bar devices in the HgTe quantum well as shown in Fig. 1(a) in the main text. We use standard optical lithography methods and follow a fabrication recipe with a two-step etching process (dry + wet) as described elsewhere [S3] to remove re-deposition and ensure smooth mesa edges. Metallic contacts are defined in a second lithography step, followed by deposition of 60 nm of AuGe eutectic alloy, also as described in [S3]. Finally, a 40 nm aluminum oxide dielectric layer is grown by atomic layer deposition, and a narrow (2 $\mu$m wide) gate defined in the last optical lithography step, followed by electron beam deposition of Ti/Au 5/50 nm (inset of Fig.1(c) and Fig. S1).

Magneto-transport data were recorded at 2.1 K in a He-3 cryostat. Resistance measurements were performed using an AC lock-in constant voltage technique, with an excitation voltage of 200 $\mu$V amplitude, 7 Hz frequency.

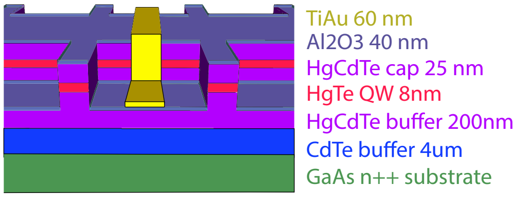


FIG. S1. Sketch of the layer structure of the device. From bottom to top: Doped GaAs n + + is used as a substrate. A buffer layer of 4 $\mu$m of CdTe is grown above it, with sufficient thickness to allow for full lattice relaxation. Successive epitaxial layers thus grow strained to the CdTe lattice constant: a buffer layer $Hg_{0.3}Cd_{0.7}Te$ of 100 nm, the HgTe quantum well with thickness $8 \pm 0.5$ nm determined by x-ray reflectometry and finally a cap layer of 25 nm of $Hg_{0.3}Cd_{0.7}Te$. The conductive substrate can be used as a backgate electrode with the CdTe layer acting as dielectric.

## S2. Capacitor model for carrier density estimation

Carrier densities have been estimated using a simple capacitor model. The capacitance for the backgate dielectric $C_{\rm bg}$ is extracted from Hall measurements in the non-topgated area $1.4 \times 10^{10}$ cm$^{-2}$/V. Carrier density under the topgate is defined by the expression $n_{\rm tg} = C_{\rm bg}(V_{\rm bg} - V_{\rm bg0}) + C_{\rm tg}(V_{\rm tg} - V_{\rm tg0})$ so that the topgate zero-density line follows:

$$(V_{\rm tg} - V_{\rm tg0}) = -(C_{\rm bg}/C_{\rm tg})(V_{\rm bg} - V_{\rm bg0}) \qquad \text{(S1)}$$

As described in the main text and in Fig. 1(b), the $V_{\rm tg}$ position of the maximum of resistance has been fit to this line. From this fit, we extract the ratio between topgate and backgate capacitances to be $C_{\rm tg}/C_{\rm bg} \simeq 30$. This yields $C_{\rm tg} = 4.2 \times 10^{11}$cm$^{-2}$/V, within expected values of capacitance for the 40 nm $Al_2O_3$ topgate dielectric layer.

## S3. Calculation of the quantum well band structure

The band structures shown in Fig. 3(a) of the main text were computed with the standard Bernevig-Hughes-Zhang effective model for HgTe quantum wells. The parameters used are given in Table I and were obtained by fitting a full 8-band Kane model. To compute the bands of a finite sample in magnetic fields, we discretize the

| $A$ (eVÅ) | $B$ (eVÅ$^2$) | $C$ (eV) | $D$ (eVÅ$^2$) |
|---|---|---|---|
| 3.572 | -77.6 | 0 | -60.2 |
| $M$ (eV) | $\Delta$ (eV) | $g_{E\perp}$ | $g_{H\perp}$ |
| -0.008 | 0.0015 | 24.8 | -1.21 |

TABLE I. BHZ model parameters for a 7.5 nm wide strained HgTe quantum well.

BHZ model on a lattice in the usual way, and add a vector potential via minimal substitution. X-ray reflectometry measurements give a quantum well width of $8 \pm 0.5$ nm. We have used parameters for a 7.5 nm well, within the experimental uncertainty of our measured width. The critical field in this case is 3.8 T, consistent with our results. For comparison, the critical field for the 8 nm well calculated in the same way is around 5 T. While it is difficult to predict the critical field exactly with the uncertainty of experimentally measured parameters, this calculation is qualitatively consistent with the critical field being between the values of 3 T and 5 T probed in the experiment.

Note the parameter $A$ in Table I can be taken as the bulk Fermi velocity ($A/\hbar \approx 5.4\times10^5$ m/s), so an estimate of the decay length into the bulk of evanescent modes is given by $\hbar v_F/2M = A/2M = 22$ nm as stated in the main text.

## S4. Estimate of equilibration length

In the unipolar $nn'n$ regime, when the conduction band is populated, we observe conductance plateaus that are consistent with full equilibration between all edge modes. In the BHZ model the conservation of $s_z$ only allows modes with the same spin to equilibrate, but spin mixing becomes possible once inversion symmetry breaking is included in the model. For the conduction band of inverted HgTe quantum wells, which is of H1 character, bulk inversion asymmetry (BIA) induces a spin splitting that is linear in momentum [S4], while structural inversion asymmetry (SIA) induces a cubic splitting [S5, S6] which we neglect. The conduction band effective Hamiltonian can be obtained in perturbation theory from the BHZ model [S6] and takes the form

$$H = \frac{\hbar^2 k^2}{2m} + \alpha\hbar(\sigma_x k_y - \sigma_y k_x) + \frac{1}{2}(g_{H1}\mu_B + g\mu)\sigma_z H \quad \text{(S2)}$$

where $m = \hbar^2(2B - 2D - A^2/M)^{-1} \approx \hbar^2 M/A^2$ in terms of the BHZ parameters and $\mu_B = e\hbar/2m_e$ is the Bohr magneton. The coupling $\alpha$ can be computed in perturbation theory in the BIA strength $\Delta$ and to first order is given by $\alpha = \Delta A/(\hbar M)$. Besides the original BHZ Zeeman coupling for the H1 band, $g_{H1}\mu_B$, there is an extra contribution to the Zeeman term $g\mu = 2(e\hbar/2m)$ obtained from the projection to the conduction band. This is the usual term obtained when taking the non-relativistic limit of a Dirac equation. Since with our BHZ parameters $m = 0.005 m_e$, this term always dominates and $\mu_B$ can be neglected.

The equilibration length for our system can be estimated by adapting the theory developed in Ref. S7. Assuming scattering originates from screened Coulomb impurities in the 2DEG plane, and considering only the lowest Landau level, the inverse scattering length is given by

$$l^{-1} = \frac{(2\pi)^{3/2}}{v_1 v_2}\left(\frac{e^2}{\hbar\epsilon}\right)^2 \frac{N}{q_s^2\lambda}\left[\frac{m\delta v\alpha g\mu H}{\delta E^2}\right]^2 \quad \text{(S3)}$$

where $v$ is the edge state velocity in the spinless problem, $v_{1,2}$ are the velocities of the spin-split edge states and $\delta E = 2\sqrt{(g\mu H/2)^2 + (mv\alpha)^2}$ is their energy splitting, $\delta v = v_2 - v_1$, N is the impurity density, and $q_s$ is the inverse screening length. This expression is valid in the conditions $\delta k \ll \lambda^{-1} \ll q_s$, where $\delta k \approx \delta E/v$ is the momentum separation of the spin-split edge states and $\lambda = \sqrt{\hbar c/eB}$ is the magnetic length.

A model for the edge potential is required to estimate the edge velocities. Using a parabolic potential, in Ref. S7 it is estimated that $\delta v/v \approx \delta E/\hbar\omega_c$ with $\omega_c = eH/m$. The value of $v$ will depend on details of the potential but a typical edge state velocity in the QH regime is [S8] $v = 10^5$ m/s. We also assume that $\delta v \ll v$ so $v_1 v_2 \approx v^2$. For the screening length we take the Thomas-Fermi approximation [S9], $q_s = (2\pi e^2/\epsilon)(m/\pi\hbar^2)$. We finally get

$$l^{-1} = (2\pi)^{3/2}\frac{N}{\lambda}\frac{\hbar^2}{4m^2}\left[\frac{m\alpha g\mu H}{\hbar\omega_c\delta E}\right]^2 = \frac{(2\pi)^{3/2}N\hbar^2\alpha^2}{4\delta E^2}\frac{1}{\lambda} \quad \text{(S4)}$$

Previous transport experiments in HgTe [S10] estimate a density of impurities up to $N = 10^{11}$ cm$^{-2}$. Taking $H = 2$ T, $\lambda(2T) = 18.4$ nm we obtain $l \approx 2.3$ $\mu$m. This is indeed smaller than the width of the Hall bar of 10 $\mu$m, which is consistent with the observation of full equilibration.

## S5. Fabry-Perot oscillations at zero field

A detailed look to the data presented in Fig. 1(b) from the main text reveals the existence of oscillations in the resistance as function of $V_{tg}$, which are highlighted in Fig. S2(a), where a smoothed background is removed. In order to account for the steep variations of resistance near the gap, we use a locally weighted 2nd degree polynomial regression method [S11] with a span of 0.1 V.

A zoom on those oscillations in the $p$-$n$-$p$ quarter is shown in Fig. S3(a). In this region, oscillations present

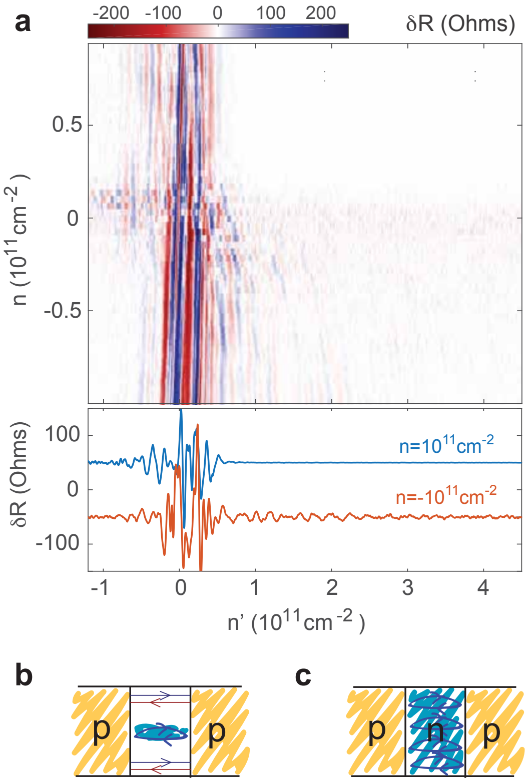


FIG. S2. (a) Top: Oscillations in the resistance across the junction ($\delta R$) are visible after removing a smoothed resistance background. Bottom: Horizontal linecuts from the very top and bottom of the 2D color map, at $n = 10^{11}$ cm$^{-2}$ (blue, upper trace) and $n = -10^{11}$ cm$^{-2}$ (orange, lower trace). Data are shifted vertically for clarity. (b),(c) Sketch of different scenarios for Fabry-Perot interference: in the p-gap-p regime (b), where due to inhomogeneity of the material, certain areas of the topgated region remain non-gapped and collimation results in increased intensity; and in the *p*-*n*-*p* quadrant (c).

a peak to peak intensity of about 10-20 Ohms. They are clearly periodic with the density of carriers under the top-gated area ($n'$) and present a slight dependence on the density in the outer region ($n$). This behavior resembles the one reported for a bipolar 2DEG in graphene [S12, S13]. According to those works, oscillations originate from the constructive Fabry-Perot interference of electrons confined by the potential barriers on both sides of the junction, as sketched in Fig. S2(c).

In a particle-in-a-box model, the oscillations period depends on the carrier density as $\Delta(n') \simeq \sqrt{g\pi n'}/L$, where $L$ is the topgate length and $g$ the degeneracy of charge carrier energy states. The fit of the periodicity of our data to this model in the region where oscillations appear more clearly ($n'$ from 0.5 to $5 \times 10^{11}$ cm$^{-2}$) is shown in Fig. S3(b) and yields an effective length for the channel $L^* = 0.6 \pm 0.1$ $\mu$m, shorter than the physical length of the topgate electrode.

While oscillations are expected in the *p*-*n*-*p* and symmetrically in the *n*-*p*-*n* region, it is remarkable that they also appear, with even higher intensity, when the central region approaches zero density.In this region, which we refer to as *p*-gap-*p*, oscillations only depend on $n'$ and present a periodicity which is similar to the ones in the *p*-*n*-*p* region within error. They are however about ten times more intense, with an averaged intensity of 100 $\omega$. Since elastic scattering is forbidden in QSH states as long as TRS applies, the oscillations present around zero density could not be in principle the result of constructive interference on the QSH states backscattering at the leads [S14]. While two-electron inelastic processes are still possible, they could not account for such high signal intensity.

The low resistance observed in the gap (Fig. 1(b) main text, linecut 1), well below the expected quantized value coming from edge transport, suggests that the bulk may not be fully insulating due to inhomogeneity of the material. If the disorder-induced potential fluctuations are of the order of the bulk gap, when the topgate voltage lowers the electron density from the $p$ side, the junction will first present electron and hole puddles among insulating regions, before the hole puddles eventually merge into an $n$-doped region. Assuming the potential fluctuates on a scale $\xi \sim 1$ $\mu m > L$, the insulating regions are always short-circuited by puddles and the resistance is generally lower than the expected quantized value. In this scenario, sketched in Fig. S2(b), oscillations can be observed as soon as the first $n$-like puddle is generated, which generates an effective *p*-*n*-*p* junction of much smaller width. The higher intensity of the oscillations in this regime would be explained by the better collimation produced by a shorter width. This intensity increase is gradually lost as the $n$ puddles become larger and larger. These oscillations might share a common origin with the fluctuations frequently reported in transport measurements in HgTe quantum wells in the QSH regime [S15–S19].

It is worth also mentioning here that bulk states for band inverted material have been predicted to extend larger distances into gapped areas than for the non-

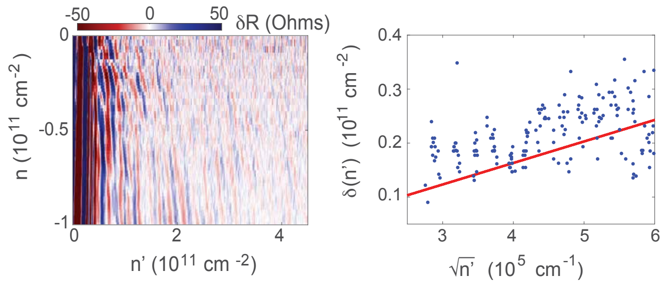


FIG. S3. (a) Zoom into resistance oscillations for the *p*-*n*-*p* region. (b) Resistance oscillations period in density $\delta n'$ obtained as distance between contiguous maxima as a function of $(n')^{1/2}$ for the region in (a): the bipolar *p*-*n*-*p* quadrant. In red, a linear fit of the data.

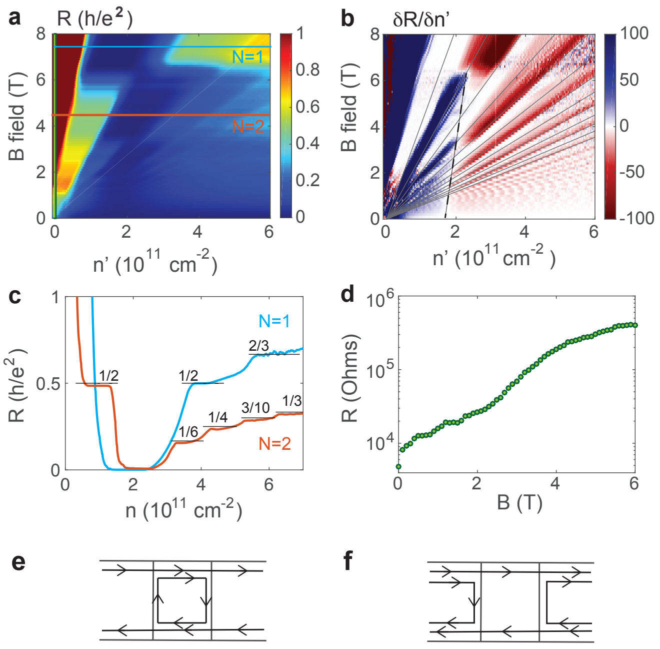


FIG. S4. (a) 4-terminal resistance $R$ measured at constant $V_{bg} = 11$ V ($n = 1.5 \times 10^{11}$ cm$^{-2}$) as a function of $V_{tg}$ and $B$-field. (b) Gradient of resistance as a function of density in the central region ($n'$). Expected positions for both semi-integer and integer filling factor $\nu'$ values are marked with continuous black lines. The dotted line separates the density regions such that $N > N'$ on the left and $N' > N$ on the right. (c) Linecuts from (a) at $B = 4.5$ T and $B = 7.8$ T. (d) Linecut from (a) following the zero density $n' = 0$ line. (e),(f) Sketches for the edge structure on the $N' > N$ and the $N > N'$ regimes, respectively.

inverted semiconductor counterpart [S20, S21]. However, these effects are relevant for transport when the length of the junction is small compared to the decay length of the evanescent modes $L \leq v_F/2M$. Our experiment is rather in the opposite regime since $L \sim 500$ nm, while $v_F/2M \sim 22$ nm as estimated from the effective model for the quantum well.

### S6. Details on the QH regime

Already in Fig. 2(a) on the main text, we observe that the resistance tile corresponding to $N = 1, N' = 1$ appears to be much larger than the contiguous one for $N' = 2$. To further understand this, in Fig. S4(a) we plot resistance as a function of both $n'$ and applied $B$-field, while the outer region density is kept at constant $n = 1.5 \times 10^{11}$ cm$^{-2}$. The transition from $N' = 1$ to 2 plateaus occur differently in the two curves depicted in Fig. S4(c), which are horizontal linecuts at constant field, such that $N = 1$ (cyan), $N = 2$ (red) respectively. In the $N = 1$ linecut, the transition between the $N' = 1$ ($R = 0$) and the $N' = 2$ ($R = 1/2h/e^2$) plateau spreads over a broad range of densities and the second plateau appears as a consequence narrower than the first. In comparison, in the $N = 2$ case, the same transition (from $N' = 1$ ($R = 1/2$) to $N' = 2$ ($R = 0$)) it is rather abrupt. If we now look at the gradient of resistance as a function of density $\delta R/\delta n'$ in Fig. S4(b) we can observe this is a general behavior for two differentiated regions (separated by a dashed line). It is relevant to point out here that the left region corresponds to densities such that $\nu' < \nu$, while on the right $\nu' > \nu$. In the left region, transitions between plateaus appear as negative $\delta R/\delta n'$ areas, are sudden and occur around semi-integer filling values $\nu'$. In contrast, in the $\nu' > \nu$ region, $\delta R/\delta n'$ is positive between plateaus, transitions spread over a larger range of $n'$ and the final resistance plateau is only reached near the next integer value of $\nu'$.

This could be a consequence of the particular geometry of our device. The central region of our junction has a high aspect ratio, $L = 2.5$ $\mu$m by $W = 10$ $\mu$m, even higher if we consider the effective length of $L* = 0.6$ $\mu$m extracted in section S2. On the one hand, for $N' \leq N$ the device is in the so-called *edge transmission* regime [S22]. $N'$ edge states will perfectly transmit through the junction and the rest $N - N'$ would be reflected, as sketched in Fig. S3(f). On the other hand, for $N' > N$, the device is in the *equilibration* regime: the current carried by the $N$ outer modes is equally distributed between the $N'$ modes propagating at the central area of the junction. Since edge states corresponding to higher filling factors are spatially located at inner positions of the sample, the geometry of our junction may prevent a good matching between the edge states at the different regions of the junction. Thus a higher carrier density is required in order to reach the fully equilibrated situation, where transmission occurs into all $N'$ modes, and a plateau appears.

Finally, Fig. S4(d) shows the evolution of the resistance at zero density in the junction (the outer region is highly doped so that it can be considered as a lead) as a function of the magnetic field. As the field increases, resistance rises well above $h/e^2$. This matches expectations for QSH states where scattering protection has been lifted, and also indicates that bulk states are already well-localized at applied fields of a few hundred mT. Bulk localization at 3T is further indicated by the quantized resistance shown in Fig.3 (main text) for N=1: bulk conduction would cause departure from the quantized plateau values.

### S7. Edge states 1D capacitance

Whereas the 2D carrier density ($n$) can be easily estimated by means of a simple capacitor model, estimating how the gate voltage changes $n_{1D}$ is not trivial. In a simple approximation and for a particle-in-the-box model, in one dimension, one would expect the period of Fabry-Perot oscillations to be constant and given by

$\delta(n_{1D}) = g/L$, where $g$ is the state degeneracy and $L$ the length of the junction. Assuming $g = 2$, $L = 0.6$ $\mu$m, and $\delta(V_{\rm tg}) \simeq 0.024$ V being the resistance oscillation voltage period of our data, we infer a one-dimensional capacitance for the edge mode of $C_{\rm 1D} = \delta(n_{1D})/\delta(V_{\rm tg}) \simeq 1.4 \times 10^6$ cm$^{-1}$V$^{-1}$

---

* E-mail: rcalvo@nanogune.eu or mreyescalvo@gmail.com
† Present address:Rudolf Peierls Centre for Theoretical Physics, Oxford University, UK
‡ E-mail: goldhaber-gordon@stanford.edu
[S1] P. Leubner, L. Lunczer, C. Brüne, H. Buhmann, and L. W. Molenkamp, Phys. Rev. Lett. **117**, 086403 (2016).
[S2] E. G. Novik, A. Pfeuffer-Jeschke, T. Jungwirth, V. Latussek, C. R. Becker, G. Landwehr, H. Buhmann, and L. W. Molenkamp, Phys. Rev. B **72**, 035321 (2005).
[S3] E. Y. Ma, M. R. Calvo, J. Wang, B. Lian, M. Mühlbauer, C. Brüne, Y.-T. Cui, K. Lai, W. Kundhikanjana, Y. Yang, *et al.*, Nat. Comms. **6** (2015).
[S4] R. Winkler, Phys. Rev. B **62**, 4245 (2000).
[S5] Y. S. Gui, C. R. Becker, N. Dai, J. Liu, Z. J. Qiu, E. G. Novik, M. Schäfer, X. Z. Shu, J. H. Chu, H. Buhmann, and L. W. Molenkamp, Phys. Rev. B **70**, 115328 (2004).
[S6] D. Rothe, R. Reinthaler, C. Liu, L. Molenkamp, S. Zhang, and E. Hankiewicz, New J. Phys. **12**, 065012 (2010).
[S7] A. V. Khaetskii, Phys. Rev. B **45**, 13777 (1992).
[S8] D. T. McClure, Y. Zhang, B. Rosenow, E. M. Levenson-Falk, C. M. Marcus, L. N. Pfeiffer, and K. W. West, Phys. Rev. Lett. **103**, 206806 (2009).
[S9] T. Ando, A. B. Fowler, and F. Stern, Rev. Mod. Phys. **54**, 437 (1982).
[S10] G. Tkachov, C. Thienel, V. Pinneker, B. Büttner, C. Brüne, H. Buhmann, L. W. Molenkamp, and E. M. Hankiewicz, Phys. Rev. Lett. **106**, 076802 (2011).
[S11] For details see `https://es.mathworks.com/help/curvefit/smoothing-data.html`.
[S12] A. F. Young and P. Kim, Nature Physics **5**, 222 (2009).
[S13] A. Varlet, M.-H. Liu, V. Krueckl, D. Bischoff, P. Simonet, K. Watanabe, T. Taniguchi, K. Richter, K. Ensslin, and T. Ihn, Phys. Rev. Lett. **113**, 116601 (2014).
[S14] L. B. Zhang, F. Zhai, and K. Chang, Phys. Rev. B **81**, 235323 (2010).
[S15] M. König, S. Wiedmann, C. Brüne, A. Roth, H. Buhmann, L. W. Molenkamp, X.-L. Qi, and S.-C. Zhang, Science **318**, 766 (2007).
[S16] M. König, H. Buhmann, L. W. Molenkamp, T. Hughes, C.-X. Liu, X.-L. Qi, and S.-C. Zhang, J. Phys. Soc. Jpn. **77**, 031007 (2008).
[S17] A. Roth, C. Brüne, H. Buhmann, L. W. Molenkamp, J. Maciejko, X.-L. Qi, and S.-C. Zhang, Science **325**, 294 (2009).
[S18] G. Grabecki, J. Wróbel, M. Czapkiewicz, S. Gierałtowska, E. Guziewicz, M. Zholudev, V. Gavrilenko, N. Mikhailov, S. Dvoretski, F. Teppe, *et al.*, Phys. Rev. B **88**, 165309 (2013).
[S19] G. Gusev, Z. Kvon, O. Shegai, N. Mikhailov, and S. Dvoretsky, Solid State Commun. **205**, 4 (2015).
[S20] E. G. Novik, P. Recher, E. M. Hankiewicz, and B. Trauzettel, Phys. Rev. B **81**, 241303 (2010).
[S21] R. Reinthaler and E. Hankiewicz, Phys. Rev. B **85**, 165450 (2012).
[S22] B. Özyilmaz, P. Jarillo-Herrero, D. Efetov, D. A. Abanin, L. S. Levitov, and P. Kim, Phys. Rev. Lett. **99**, 166804 (2007).
